# Supplementary material for: AtomoVideo: High Fidelity Image-to-Video Generation
Source: arXiv:2403.01800 source file (2024-03-05)
Supplement: Supplementary file 1 [file 7_Supp.tex]

\section{Comparison Details}

To ensure fairness, we utilized the official open-source code and parameters provided for all comparison methods. 
Specifically, for all models, we employed the CLIP text encoder \cite{8_CLIP_RadfordKHRGASAM21} to get the text embedding, and the VAE model and parameters officially provided by ``stable-diffusion-v1-5" \cite{7_SD_RombachBLEO22} to encode the input image into the latent space. The image $I \in \mathbb{R}^{3\times{H}\times{W}}$ will be converted to the $z^0\in \mathbb{R}^{4\times{\frac{H}{8}}\times{\frac{W}{8}}}$.
(1) \textit{SDEdit}~\cite{16_SDEdit_MengHSSWZE22}, we firstly noised the encoded image latent with the initially sampled noise (using Equation \text{\color{Red}2} in the main text). The noisy latent will be used for the denoising steps in the reverse process.
(2) \textit{ConcateImage}, we concatenated the image latent with the sampled noise through the feature channel, thus resulting the noisy latent $z_T^{0:L-1}\in\mathbb{R}^{L\times8\times{\frac{H}{8}}\times{\frac{W}{8}}}$. Therefore, beyond the 
parameters of VAE and text encoder, the remaining parameters within the framework require fine-tuning. We fine-tuned on WebVid10M Dataset \cite{60_WebVid_bain2021frozen} using the Adam optimizer with a learning rate of 1e-5 for one epoch.
(3) \textit{ControlNet Reference-Only}~\cite{12_ControlNet_zhang2023adding}, we utilized the ``reference-only" processor which directly linked the attention layers of SD to the input image. 
(4) \textit{IP-Adapter}~\cite{14_IP-Adapter_ye2023ip-adapter}, 
we utilized the official ``IP-Adapter Plus" version which extracted the fine-grained image features to get better performance.
(5) \textit{VideoCrafter1-I2V}~\cite{35_VideoCrafter_chen2023videocrafter1}, we directly utilzed the Image2Video model in the released project.
(6) \textit{VideoComposer}~\cite{36_VideoComposer_2023videocomposer}, we both utilized the ``style" and ``single image" mode for the input image.
(7) \textit{I2VGen-XL}~\cite{37_I2VGen-XL_zhang2023i2vgenxl}, 
we used the initial version model which had been open-sourced on the Modelscope platform.
For our methods \textit{Ours} and \textit{Ours+IP-Adapter~\cite{14_IP-Adapter_ye2023ip-adapter}}, as well as $(1)\sim(4)$, we all adopted the pre-trained VLDM (including the ``Realistic Vision V2.0" model and motion module ``mm\_sd\_v15\_v2" in the AnimateDiff~\cite{25_animatediff_guo2023animatediff}. In order to maintain consistency with the official project implementation, the shorter side of input image is resized to 256 for \textit{VideoComposer}~\cite{36_VideoComposer_2023videocomposer} and \textit{I2VGen-XL}~\cite{37_I2VGen-XL_zhang2023i2vgenxl}, 320 for \textit{I2VGen-XL}~\cite{37_I2VGen-XL_zhang2023i2vgenxl} and 512 for other comparison methods. For all generated videos, we all take the length as $L=16$.

\section{Limitations and Society Impacts}
%动效强度不够，长度还不够长, 控制性还不够（社会伦理）
Although our method has effectively improved fidelity in image-to-video generation, there are still some limitations. (1)  Motion intensity. Our method currently is not sufficient for generating larger-scale motion effects. While there is a trade-off between the intensity of motion and fidelity, future work may consider how to increase the magnitude of the motion while preserving the image identity and frame consistency. (2) Video length. Our work, as well as most existing work, is not yet capable of generating longer videos, which poses significant challenges to the maintenance of inter-frame consistency and the ability of storytelling. (3) Controllability. Our method is primarily used for image-to-video generation, aiming to animate still images. However, the current ability to precisely control motion effects in generated videos is still lacking, which may lead to uncertainty in the video output and potential social and ethical risks. In future work, we will focus on enhancing the ability to control the generated video.
